# Supplementary material for: T3VIP: Transformation-based 3D Video Prediction
Source: arXiv:2209.11693 source file (2022-09-19)
Supplement: Supplementary file 1 [file 7_Appendix.tex]

%%%%%%%%%% Merge with supplemental materials %%%%%%%%%%
\clearpage

\setlength{\belowcaptionskip}{0pt}

\begin{strip}
\begin{center}
\vspace{-5ex}
\textbf{\LARGE \bf T3VIP: Transformation-based 3D Video Prediction} \\
\vspace{2ex}

\Large{\bf- Supplementary Material -}\\
\vspace{0.4cm}
\normalsize{Iman Nematollahi, Erick Rosete-Beas, Seyed Mahdi B. Azad, Raghu Rajan, Frank Hutter, Wolfram Burgard}
\end{center}
\end{strip}

%%%%%%%%%% Merge with supplemental materials %%%%%%%%%%
%%%%%%%%%% Prefix a "S" to all equations, figures, tables and reset the counter %%%%%%%%%%
\setcounter{section}{0}
\setcounter{equation}{0}
\setcounter{figure}{0}
\setcounter{table}{0}
\setcounter{page}{1}
\makeatletter

%\makeatletter \renewcommand{\fnum@figure}
%{\figurename~S\thefigure}
%\makeatother
% 
%% Hack for making figures Say \figurename S\thefigure, e.g. Figure S1:
%\makeatletter
%\makeatletter \renewcommand{\fnum@table}
%{\tablename~S\thetable}
%\makeatother

% Hack For section headers starting with S
%\renewcommand{\thesection}{S.\Roman{section}}
%\renewcommand{\thesubsection}{\thesection.\Alph{subsection}}
%\renewcommand{\bibnumfmt}[1]{[S#1]}
% citenumfont command adds S to all numbers
%\renewcommand{\citenumfont}[1]{\textit{S#1}}
%\renewcommand{\bibnumfmt}[1]{[S#1]}
%\renewcommand{\citenumfont}[1]{S#1}
%%%%%%%%%% Prefix a "S" to all equations, figures, tables and reset the counter %%%%%%%%%%

\normalsize

% This supplementary material provides details on the data collection environment and methodology, followed by in depth qualitative and quantitative experimental evaluations that were performed in addition to those reported in the main paper. We also present extensive ablation studies on the various architectural components of our network.

In this supplementary material, we present additional details 

\section{Video Prediction}
\subsection{Network Details}
\subsection{Additional Experiments}
\section{Hyperparameter optimization}\label{sec:append_hpo}
\subsection{Training Details}
report found hyperparameters

\section{Planning}
\subsection{Model-Predictive Control}
write down the planning algorithm

\begin{table}[htbp]
\centering
\catcode`,=\active
\def,{\char`,\allowbreak}

\begin{tabular}{p{3.5cm}<{\raggedright} p{1.5cm}<{\raggedleft} }
  \toprule
    \textbf{Hyperparameters}           & \textbf{Values}\\ 
  \midrule
    population                         & 150 \\
    minimum std                        & 0.001 \\
    maximum std                        & 1.0 \\
    elite fraction                     & 0.1 \\
    horizon                            & 5 \\
    maximum iterations                 & 5 \\
    internal momentum (alpha)          & 0.1 \\
    external momentum (beta)           & 0.5 \\
    colored noise exponent             & 2 \\
    population decay factor            & 0.9 \\
    cost function decay factor                  & 0.8 \\
  \bottomrule
\end{tabular} 
\caption{iCEM hyperparameters}
\label{tab:planner_hyper}
\end{table}
